# Supplementary material for: Test Code Generation for Telecom Software Systems using Two-Stage Generative Model
Source: arXiv:2404.09249 source file (2024-04-14)
Supplement: Supplementary file 1 [file appendix.tex]

\newpage
\newpage

% the \\ insures the section title
